# Supplementary material for: Gapless neutron superfluidity can explain the late time cooling of transiently accreting neutron stars
Source: arXiv:2403.07740 ancillary file (2024-03-12)
Supplement: Supplementary file 1 [file supplement.pdf]

**Supplemental Material**

# Gapless neutron superfluidity can explain the late time cooling of transiently accreting neutron stars

V. Allard[1] and N. Chamel[1]

[1] *Institute of Astronomy and Astrophysics, Université Libre de Bruxelles, CP 226, Boulevard du Triomphe, B-1050 Brussels, Belgium*

(Dated: March 7, 2024)

In this Supplemental Material, observational data for KS 1731−260 and MXB 1659−29 are summarized and discussed. Further details on our neutron-star cooling models and parameters estimation are given. Additional results are presented and discussed.

## CONTENTS

S.I. Observations 1

S.II. Neutron star cooling models 2
- A. Diffusion of superfluid neutrons 2
- B. Specific heat 3

S.III. Parameters estimation 4

S.IV. Results 5
- A. Neutron-star cooling models with BCS superfluidity 5
  - 1. KS 1731−260 5
  - 2. MXB 1659−29 7
- B. Neutron-star cooling models with gapless superfluidity 9
  - 1. KS 1731−260 9
  - 2. MXB 1659−29 10
- C. Neutron-star cooling models within the traditional model of accreted neutron stars 11
  - 1. KS 1731−260 11
  - 2. MXB 1659−29 13
- D. Neutron superfluidity and cooling 16

S.V. Summary of the results 17
- A. Thermodynamically consistent model 17
- B. Traditional model 18

References 18

## S.I. OBSERVATIONS

The observational cooling data after the end of the outburst of KS 1731−260 and after the two outbursts of MXB 1659−29 are summarized in Tables S1, S2 and S3 respectively.

Different values for the temperature $k_{\rm B}T_{\rm eff}^\infty$ were inferred in Ref. [3] from the last observation of MXB 1659−29 after the end of outburst I. The temperature $49.0 \pm 2.0$ eV quoted in Table S2 was obtained by fitting the spectra with an absorbed neutron star atmosphere model, in which the hydrogen column density was fixed to the value $N_H = 2.0 \times 10^{21}$ cm$^{-2}$ deduced from previous observations. This is the spectral fit shown in Fig.4 of Ref. [3] and considered in Refs. [4, 5].

It is worth pointing out that even lower temperatures were actually found in Ref. [3] considering more realistic spectral models accounting not only for the neutron-star atmosphere but also for a power-law component: $k_{\rm B}T_{\rm eff}^\infty = 45.0 \pm 3.0$ eV (with a power-law index $\Gamma = 1.5$) or $k_{\rm B}T_{\rm eff}^\infty = 43.0 \pm 5.0$ eV (with a power-law index $\Gamma = 2$). As will be shown elsewhere, such temperature drops can be naturally explained by neutron-star cooling models with gapless superfluidity but not with BCS superfluidity.

Alternatively, the higher temperature $k_{\rm B}T_{\rm eff}^\infty = 55.0 \pm 3.0$ eV, more in line with predictions from standard cooling models, was obtained in Ref. [3] with an absorbed neutron star atmosphere model by allowing $N_H$ to vary (the

TABLE S1: Inferred effective surface temperature $T_{\rm eff}^{\infty}$ (as seen by an observer at infinity) of KS 1731−260 at different times after outburst from Ref. [1]. Time is given in terms of modified Julian date (MJD). The outburst ended at time $t_0 = 51930.5$. The temperature and the uncertainties at the 68% credibility level are given in electronvolts ($k_{\rm B}$ denotes Boltzmann constant).

| | Observatory | Obs ID | MJD | $k_{\rm B}T_{\rm eff}^{\infty}$ (eV) |
|---|---|---|---|---|
| 1 | Chandra | 2468 | 51995.1 | 104.6±1.3 |
| 2 | XMM-Newton | 013795201/301 | 52165.7 | 89.5±1.03 |
| 3 | Chandra | 3796 | 52681.6 | 76.4±1.8 |
| 4 | Chandra | 3797 | 52859.5 | 73.8±1.9 |
| 5 | XMM-Newton | 0202680101 | 53430.5 | 71.7±1.4 |
| 6 | Chandra | 6279/5486 | 53512.9 | 70.3±1.9 |
| 7 | Chandra | 10037/10911 | 54969.7 | 64.5±1.8 |
| 8 | Chandra | 16734/17706/707 | 57242.1 | 64.4±1.2 |

TABLE S2: Same as Table S1 after the end of the 1999-2001 outburst of MXB 1659−29 (referred to as outburst I). The first six points come from Ref. [2] while the last point is from the spectral fits of Ref. [3] for an absorbed neutron star atmosphere with a fixed hydrogen column density. The outburst ended at time $t_0 = 52162$. Uncertainties are given at the 90% credibility level.

| | Observatory | Obs ID | MJD | $k_{\rm B}T_{\rm eff}^{\infty}$ (eV) |
|---|---|---|---|---|
| 1 | Chandra | 2688 | 52197.7 | 111.1±1.3 |
| 2 | Chandra | 3794 | 52563.0 | 79.5±1.6 |
| 3 | XMM-Newton | 0153190101 | 52711.6 | 73.0±1.9 |
| 4 | Chandra | 3795 | 52768.7 | 67.8±2.1 |
| 5 | Chandra | 5469/6337 | 53566.4 | 55.5±2.4 |
| 6 | Chandra | 8984 | 54583.8 | 54.8±3.2 |
| 7 | Chandra | 13711/14453 | 56113 | 49.0±2.0 |

best fit value for this observation is $N_H = (4.7 \pm 1.3) \times 10^{21}$ cm$^{-2}$). However, large variations of $N_H$ are rather unexpected unless the accretion disk was precessing [3]. Despite the lack of observational evidence, the authors of Ref. [2] *assumed* this scenario to be more likely, and discarded the last observations of MXB 1659−29 after the end of outburst I considering that the crust had reached thermal equilibrium with the core. In this scenario, the cooling curve can be explained with BCS superfluidity, both within the traditional model of accreted neutron-star crusts [2, 3, 6, 7] and in the thermodynamically consistent approach that accounts for neutron diffusion [8]. We have checked that observations could also be reproduced with gapless superfluidity. In this case, the physical interpretation of the cooling data is ambiguous. However, we would like to stress that the spectral fits of Parikh et al. [2] did not lead to any appreciable change of $N_H$ throughout the observations (see their footnote 9). This result is inconsistent with their hypothesis of accretion disk precession. Therefore, a further cooling of the neutron star appears more plausible.

## S.II. NEUTRON STAR COOLING MODELS

In this section, we provide some more details on the microphysics inputs of our neutron star cooling models.

### A. Diffusion of superfluid neutrons

Neutron star cooling simulations of quasipersistent soft X-ray transients generally rely on the accreted-crust model of Haensel and Zdunik [9] according to which nuclei undergo electron captures, neutron captures and emissions, and possibly pycnonuclear fusion reactions as they slowly sink inside the star. These reactions are expected to release $Q_{\rm nuc} \approx 0.3$ MeV/nucleon in the outer crust and $Q_{\rm nuc} \approx 1.5$ MeV/nucleon in the inner crust (so called 'deep crustal heating' paradigm). Free neutrons are implicitly assumed to move with nuclei. However, Gusakov and Chugunov [10, 11] have recently shown that this assumption is unrealistic. They have found that the diffusion of superfluid neutrons changes the traditional picture of accreted neutron-star crusts: 1) the equation of state turns out

TABLE S3: Same as Table S1 for MXB 1659−29 after the end of the 2015-2017 outburst (referred to as outburst II) using the data from Ref. [2]. The outburst ended at time $t_0 = 57809.7$. Uncertainties are given at the 90% credibility level.

| | Observatory | Obs ID | MJD | $k_{\rm B}T_{\rm eff}^{\infty}$ (eV) |
|---|---|---|---|---|
| 1 | Swift | Interval 1 | 57822.0 | 91.5±8.8 |
| 2 | XMM-Newton | 0803640301 | 57835.8 | 87.9±1.4 |
| 3 | Chandra | 19599 | 57868.0 | 82.7±2.0 |
| 4 | Chandra | 19600 | 57937.6 | 74.8±2.5 |
| 5 | XMM-Newton | 0803640401 | 57987.3 | 75.1±2.4 |
| 6 | Chandra | 19601 | 58151.5 | 66.0±3.0 |
| 7 | Chandra | 19602 | 58314.4 | 56.3±4.2 |

to be similar to that of cold catalyzed matter, 2) the heat deposited is reduced.

To account for neutron diffusion, we have modified the original `crustcool` code[1] following the prescription given in Refs. [10, 11], namely:

- we have taken the composition and the equation of state of accreted crusts to be the same as that of Haensel and Zdunik (1990) [9], for ashes made of iron, up to the point where the proton number $Z$ decreases to 20;
- we have kept the same value of $Z = 20$ in the deeper layers and we have determined the mass number $A_{\rm cl}$ of clusters so that the proton fraction $Z/A_{\rm cl}$ and the fraction of free neutrons are the same as in the catalyzed matter calculated by Douchin and Haensel [12];
- we have reduced the heat released per nucleon to $Q_{\rm nuc} = 0.1$ MeV/nucleon in the outer crust and $Q_{\rm nuc} = 0.3$ MeV/nucleon in the inner crust.

## B. Specific heat

The total specific heat of the crust is the sum of contributions from electrons, ions, and free neutrons (in the inner crust). For the first two, we use the same expressions as described in Ref. [13] and implemented in the original `crustcool` code. However, we have modified the expression of the neutron specific heat to allow for the presence of superflow and gapless superfluidity. These effects are taken into account via the reduction factors introduced in the paper.

In the absence of superflow $\mathbb{V}_n = 0$, which we refer to as the BCS state, the reduction factor is explicitly given by [14]

$$R_{00}^{\rm (BCS)}(T/T_{cn}^{(0)}) = \left[0.4186 + \sqrt{1.007^2 + (0.5010 u_n)^2}\right]^{5/2} \exp\left(1.456 - \sqrt{1.456^2 + u_n^2}\right) , \tag{S.1}$$

where $u_n$ is defined as

$$u_n = \sqrt{1 - \frac{T}{T_{cn}^{(0)}}} \left(1.456 - 0.157\sqrt{\frac{T_{cn}^{(0)}}{T}} + 1.764\frac{T_{cn}^{(0)}}{T}\right) . \tag{S.2}$$

The neutron superfluid critical temperature $T_{cn}^{(0)}$ is shown in Fig. S1 as a function of the average mass density $\rho$ in the inner crust and core of accreted neutron stars. We have made use of the BCS relation $k_{\rm B}T_{cn}^{(0)} = \exp(\gamma)\Delta_n^{(0)}/\pi \simeq 0.56693\Delta_n^{(0)}$ with the $^1{\rm S}_0$ pairing gaps $\Delta_n^{(0)}(k_{Fn})$ predicted by different many-body methods. For any given mass density $\rho$, we have determined the neutron Fermi wave number $k_{Fn}$ from the thermodynamically consistent accreted crust composition. For comparison, we have also plotted in the same figure the critical temperatures from the empirical gaps introduced in Ref. [15].

[1] `https://github.com/andrewcumming/crustcool`

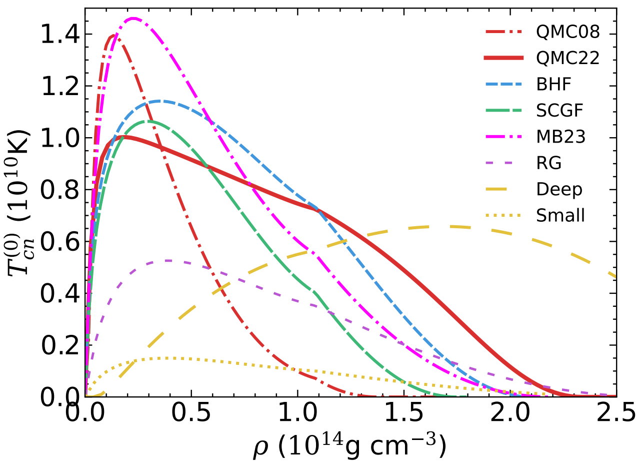


FIG. S1: ${}^1S_0$ neutron superfluid critical temperature $T_{cn}^{(0)}$ (in $10^{10}$ K) as a function of the average mass density $\rho$ (in g cm$^{-3}$) in the inner crust and core (shaded area) of accreted neutron stars using the composition of Refs. [10, 11] and the pairing gaps $\Delta_n^{(0)}$ predicted by renormalization group [16] (RG), quantum Monte Carlo calculations from 2008 [17] (QMC08) and 2022 [18] (QMC22), Brueckner Hartree-Fock theory [19] (BHF), self-consistent Green function theory [20] (SCGF), and other diagrammatic calculations [21] (MB23). The dashed and dotted yellow curves correspond to the "Deep" and "Small" gaps fine-tuned in Ref. [15] to fit the cooling data of SXTs within the traditional deep crustal heating paradigm.

In the gapless state $\mathbb{V}_{Ln} < \mathbb{V}_n \leq \mathbb{V}_{cn}^{(0)}$, the reduction factor $R_{00}^{(\rm Gapless)}$ is essentially independent of $T$ at sufficiently low temperatures and depends on $\Delta_n^{(0)}$ only through the neutron critical effective superfluid velocity $\mathbb{V}_{cn}^{(0)}$ or equivalently Landau's velocity $\mathbb{V}_{Ln}$ [22]. For a given ratio $\mathbb{V}_n/\mathbb{V}_{Ln}$, the neutron specific heat is therefore independent of $\Delta_n^{(0)}$. For $\mathbb{V}_{Ln} \leq \mathbb{V}_n \leq 1.03\mathbb{V}_{Ln}$, we employ the following analytical formula demonstrated in Ref. [22]:

$$R_{00}^{(\rm Gapless)}(T \ll T_{cn}^{(0)}, \mathbb{V}_{Ln} \leq \mathbb{V}_n \leq 1.03\mathbb{V}_{Ln}) \approx 0.9328201\sqrt{\frac{T}{T_{cn}^{(0)}}}\,. \tag{S.3}$$

In this limiting case, the neutron specific heat thus depends on $\Delta_n^{(0)}$ through $T_{cn}^{(0)}$.

## S.III. PARAMETERS ESTIMATION

The fitting parameters of the baseline neutron-star cooling model are: 1) the impurity parameter $Q_{\rm imp}$ governing the thermal conductivity, 2) the normalized effective neutron superfluid velocity $\mathbb{V}_n/\mathbb{V}_{Ln}$ entering the neutron specific heat, 3) the temperature $T_{\rm b}$ at the bottom of the envelope at the column depth of $10^{12}$ g cm$^{-2}$ and, 4) the core temperature $T_{\rm core}$. Note that in Refs. [5, 13], $T_{\rm core}$ was not treated as a free parameter but was set from the last observation, assuming that the thermal evolution lasted long enough for the crust-core thermal equilibrium to be reestablished. To assess the sensitivity of our theoretical cooling curves to these parameters, we have performed Markov-chain Monte Carlo (MCMC) simulations. For this purpose, we have modified the `mcee.py` Python routine (provided with the original `crustcool` code and relying on the Python `emcee` package[2], see Ref. [23]) to allow for the presence of superflow. The `mcee.py` routine draws samples from the posterior probability distribution of the parameters through the generation of $n_{\rm walkers}$ Markov chains of length $n_{\rm steps}$ in the parameter space (see, e.g., Ref. [24], for more details). In practice, a first MCMC simulation is run with initial guess values for the fitting parameters of our cooling simulations chosen randomly according to uniform prior probabilities (as prescribed in Ref. [13]). The modes of the resulting posterior distributions are then used in a second MCMC simulation to refine the initial guess values chosen following a Gaussian distribution, whose mean corresponds to the extracted mode. This iterative process is

---

[2] `https://github.com/dfm/emcee`

repeated until convergence is reached according to the Gelman-Rubin criterion [25]. We have found that 25 Markov chains with a length of 2000 steps (corresponding to $5\times10^4$ samples) are typically enough to reach convergence, in the sense that the Gelman-Rubin statistics (the square root of the ratio of two estimators for the target variance) lies close to 1 (in practice $\hat{R} \lesssim 1.03$). To prevent the distributions from being contaminated by any dependence on the initial parameter values, the first 10% of the samples of the chains have been removed ("burnt-in"). The `mcee.py` routine keeps track of the $n_{\rm walkers}$ Markov chains of length $n_{\rm steps}$. The output data files are used to plot the marginalized posterior probability distributions of the parameter set as well as pairwise relationships between the various parameters, through the use of the Python `corner` package[3]. The best value of each parameter is obtained by selecting the median of the corresponding marginalized probability distribution. Uncertainties are given at the 68% uncertainty level and are determined by the 0.16−0.84 quantiles of the marginalized posterior distributions.

In all cases, the accretion rate is fixed to $\dot{m} = 10^{17}$ g/s. The neutron-star mass and radius are set to $\rm M_{NS} = 1.62M_{\odot}$ and $\rm R_{NS} = 11.2$ km respectively.

## S.IV. RESULTS

### A. Neutron-star cooling models with BCS superfluidity

In this section, we present results obtained within the thermodynamically consistent model of accreted neutron stars of Gusakov&Chugunov [10, 11] in the absence of superflow (BCS state).

#### 1. *KS 1731−260*

Figure S2 shows the marginalized posterior probability distributions of the model parameters for KS 1731−260 using the realistic neutron pairing gap of Ref. [18] (left panel). For comparison, we have also run simulations using the "Deep" gap of Ref. [15], which was empirically constructed to fit the cooling data of this source. Results are displayed in the same figure (right panel). The median values of the parameters with 68% uncertainty level are summarized in Table S4. The corresponding cooling curves are shown in the paper (and also in Fig. S3). The model with realistic pairing gap (dotted curve) yields a rather poor fit of the data. Better fits can only be achieved by artificially fine tuning the pairing gap, as illustrated using the "Deep" gap of Ref. [15].

[3] `https://github.com/dfm/corner.py`

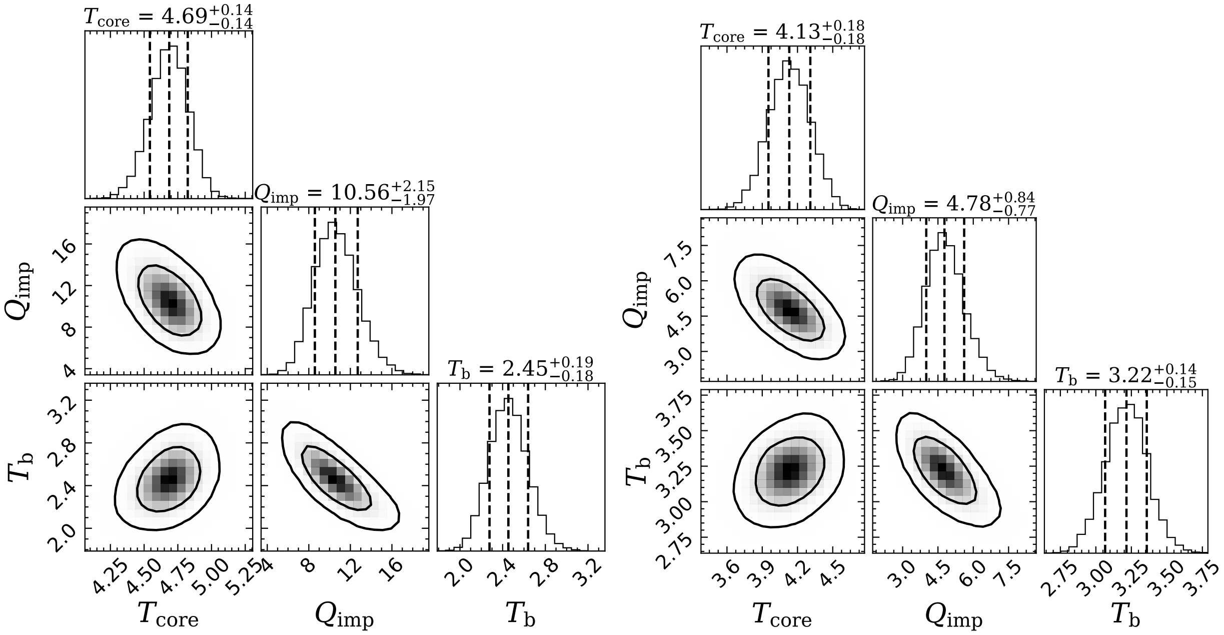


(a) QMC22 (b) Deep

FIG. S2: Marginalized 1-D and 2-D probability distributions for the parameters of our cooling model of KS 1731−260 within the model of Gusakov&Chugunov [10, 11] of accreted neutron stars in the absence of superflow (BCS state). Results were obtained using the realistic neutron pairing gap of Ref. [18] (left panel) and the fine-tuned "Deep" gap of Ref. [15] (right panel). $T_{\rm core}$ and $T_{\rm b}$ are expressed in units of $10^7$ K and $10^8$ K respectively. The dotted lines in the histograms mark the median value and the 68% uncertainty level while the contours in the 2-D probability distributions correspond to 68% and 95% credibility ranges. The cooling curves corresponding to the median values of the parameters are displayed in Fig. S3.

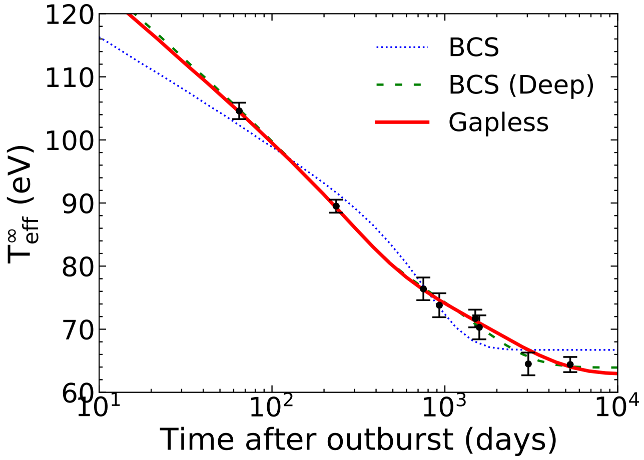


FIG. S3: Evolution of the effective surface temperature of KS 1731−260 in electronvolts (as seen by an observer at infinity) as a function of the time in days within the model of Gusakov&Chugunov [10, 11] of accreted neutron stars. Symbols represent observational data with error bars. The dotted and solid lines are models considering superfluid neutrons in the BCS and gapless states respectively using the realistic neutron pairing calculations of Ref. [18]. For comparison, results obtained with a model considering BCS superfluidity with the fine-tuned "Deep" gap of Ref. [15] are also shown (dashed line).

## 2. MXB 1659−29

Figure S4 shows the marginalized posterior probability distributions of the model parameters for the outburst I of MXB 1659−29 using the realistic neutron pairing gap of Ref. [18] (left panel) and the fine-tuned "Deep" gap of Ref. [15] (right panel). The corresponding cooling curves are shown in the left panel of Fig. S5. The model with the realistic gap fails to reproduce the last observation at $k_{\rm B}T_{\rm eff}^{\infty} = 49.0 \pm 2.0$ eV. More surprisingly, the model with the "Deep" gap does not yield satisfactory results either. This stems from the fact that this gap was empirically constructed to fit the cooling data of KS 1731−260 within the traditional model of accreted neutron stars of Haensel&Zdunik [9] (see Section *Neutron-star cooling models within the traditional model of neutron stars* below).

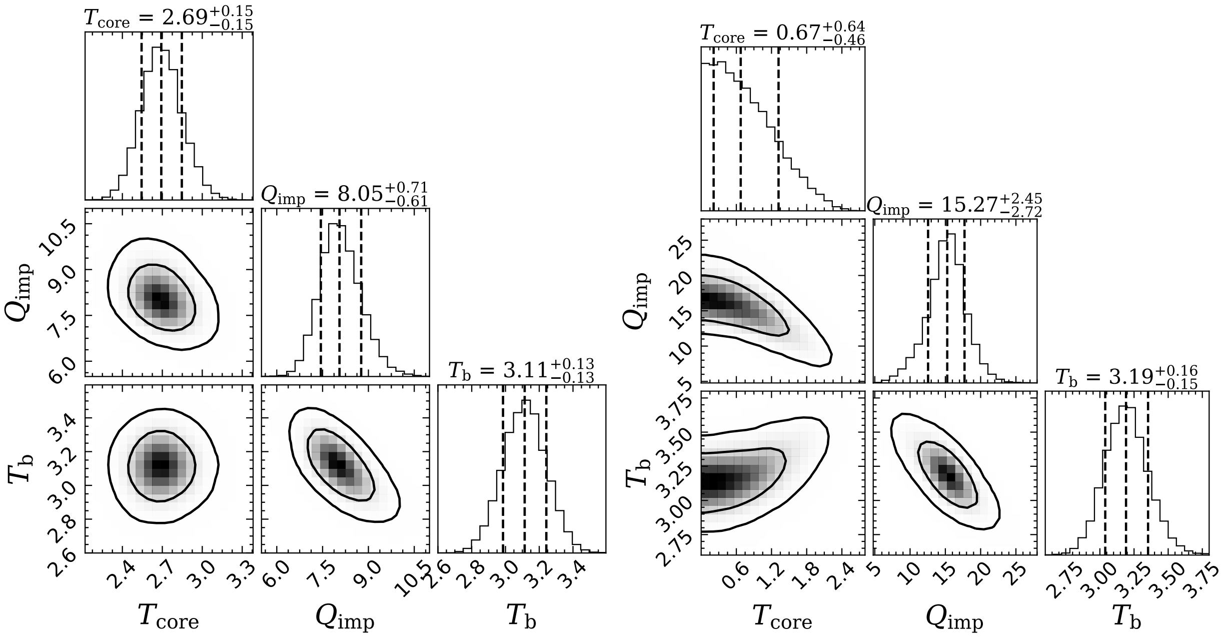


(a) QMC22 (b) Deep

FIG. S4: Marginalized 1-D and 2-D probability distributions for the parameters of our cooling model of the outburst I of MXB 1659-29 within the model of Gusakov&Chugunov [10, 11] of accreted neutron stars in the absence of superflow (BCS state). Results were obtained using the realistic neutron pairing gap of Ref. [18] (left panel) and the fine-tuned "Deep" gap of Ref. [15] (right panel). $T_{\rm core}$ and $T_{\rm b}$ are expressed in units of $10^7$ K and $10^8$ K respectively. The dotted lines in the histograms mark the median value and the 68% uncertainty level while the contours in the 2-D probability distributions correspond to 68% and 95% credibility ranges. The cooling curves corresponding to the median values of the parameters are displayed in the left panel of Fig. S5.

To check the consistency of our model, we have analyzed the outburst II keeping fixed the core temperature to the median value obtained for the outburst I [2]. Marginalized posterior probability distributions of the model parameters are shown in Fig. S6, using the realistic neutron pairing gap of Ref. [18] (left panel) and the fine-tuned "Deep" gap of Ref. [15] (right panel). As shown in the right panel of Fig. S5, the cooling data are well reproduced in both cases. The median values of the parameters for outbursts I and II with 68% uncertainty level are summarized in Table S5.

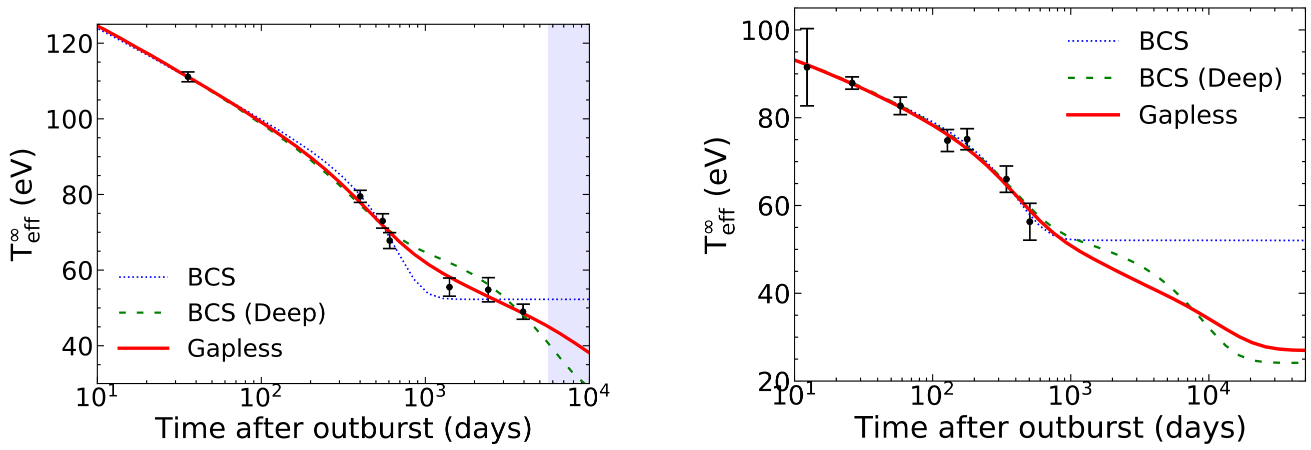


(a) Outburst I

(b) Outburst II

FIG. S5: Evolution of the effective surface temperature of MXB 1659−29 after outburst I (left panel) and outburst II (right panel) in electronvolts (as seen by an observer at infinity) as a function of the time in days within the model of Gusakov&Chugunov [10, 11] of accreted neutron stars. Symbols represent observational data with error bars. The dotted and solid lines are models considering superfluid neutrons in the BCS and gapless states respectively using the realistic neutron pairing calculations of Ref. [18]. For comparison, results obtained with a model considering BCS superfluidity with the fine-tuned "Deep" gap of Ref. [15] are also shown (dashed line). The shaded area corresponds to the second accretion phase (which occurred in 2015) and its subsequent cooling phase: the cooling curves within this region depict the expected behavior had outburst II not occurred.

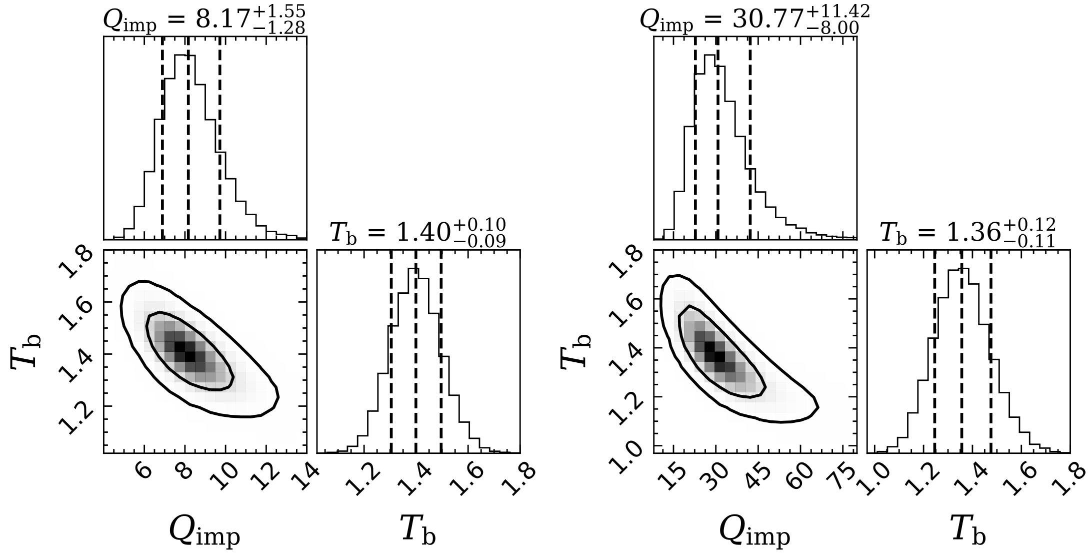


(a) QMC22

(b) Deep

FIG. S6: Same as Fig. S4 for outburst II of MXB 1659-29. The cooling curves corresponding to the median values of the parameters are displayed in the right panel of Fig. S5.

### B. Neutron-star cooling models with gapless superfluidity

In this section, we present results obtained within the model of accreted neutron stars of Gusakov and Chugunov [10, 11] suitably extended to allow for gapless superfluidity in the crust.

#### *1. KS 1731−260*

Figure S7 shows the marginalized posterior probability distributions of the model parameters for KS 1731−260 using the realistic neutron pairing calculations of Ref. [18]. The median values of the parameters with 68% uncertainty level are summarized in Table S4. The associated cooling curve is displayed in Fig. S3. Models with gapless superfluidity lead to an excellent fit to observations.

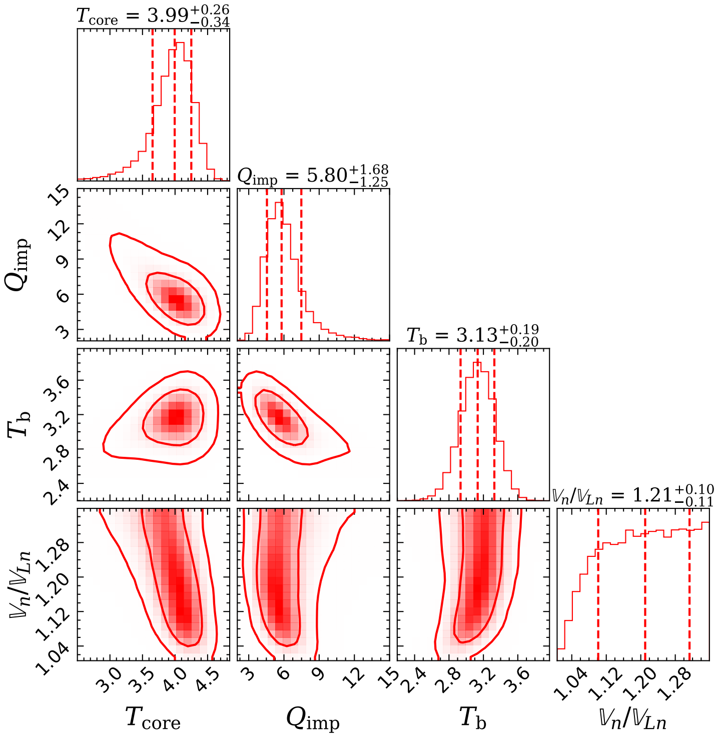


FIG. S7: Marginalized 1-D and 2-D probability distributions for the parameters of our cooling model of KS 1731−260 within the model of Gusakov&Chugunov [10, 11] of accreted neutron stars but considering gapless superfluidity, using the realistic neutron pairing calculations of Ref. [18]. $T_{\rm core}$ and $T_{\rm b}$ are expressed in units of $10^7$ K and $10^8$ K respectively. The dotted lines in the histograms mark the median value and the 68% uncertainty level while the contours in the 2-D probability distributions correspond to 68% and 95% credibility ranges. The cooling curve corresponding to the median values of the parameters is displayed in Fig. S3.

### 2. *MXB 1659−29*

The left panel of Fig. S8 shows the marginalized posterior probability distributions of the model parameters for the outburst I of MXB 1659−29 using the realistic neutron pairing calculations of Ref. [18]. The corresponding cooling curve is shown in the left panel of Fig. S5. Whereas the last point remains unexplained for cooling models assuming BCS superfluidity with realistic neutron pairing [18], allowing for the presence of superflow in the crust in the gapless state leads to an excellent fit to all the observational data.

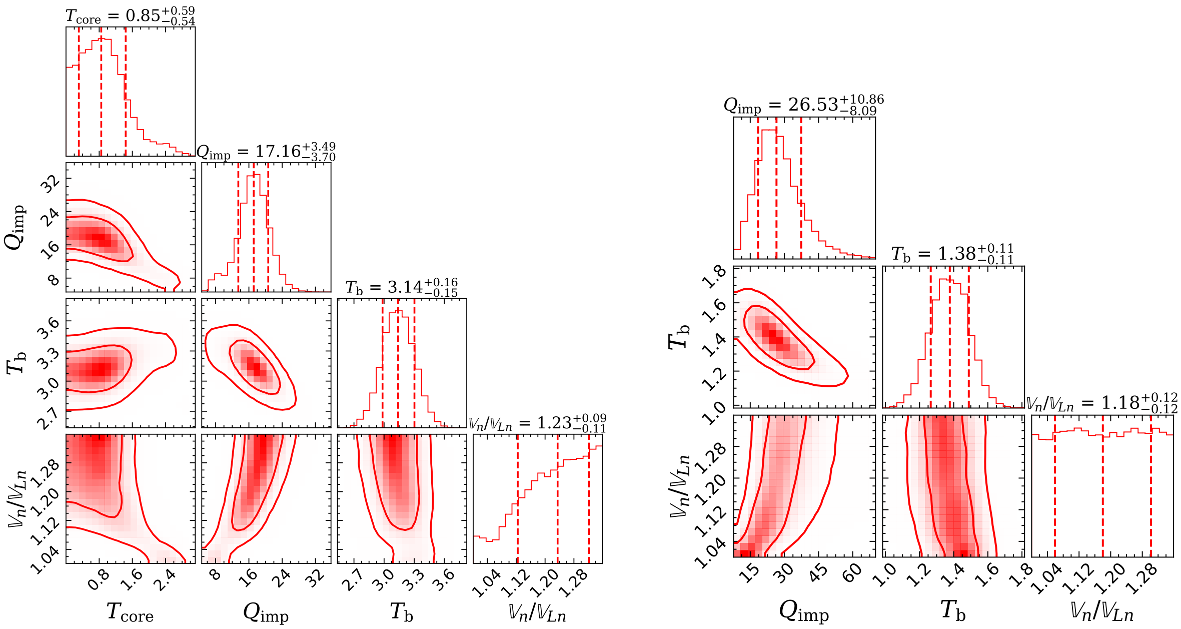


(a) Outburst I (b) Outburst II

FIG. S8: Marginalized 1-D and 2-D probability distributions for the parameters of our cooling model of the outburst I (left panel) and outburst II (right panel) of MXB 1659−29 within the model of Gusakov&Chugunov [10, 11] of accreted neutron stars in the presence of gapless superfluidity, using the realistic neutron pairing calculations of Ref. [18]. $T_{\rm core}$ and $T_{\rm b}$ are expressed in units of $10^7$ K and $10^8$ K respectively. The dotted lines in the histograms mark the median value and the 68% uncertainty level while the contours in the 2-D probability distributions correspond to 68% and 95% credibility ranges. The cooling curves corresponding to the median values of the parameters are displayed in Fig. S5.

The marginalized posterior probability distributions of the model parameters for the outburst II of MXB 1659−25, using the realistic neutron pairing calculations of Ref. [18], are shown in the right panel of Fig. S8. Following the approach of Ref. [2], these results have been obtained fixing the core temperature to the median value obtained after outburst I. We find no significant change of $Q_{\rm imp}$ and $\mathbb{V}_n$ at the 95% level, contrary to $T_{\rm b}$ (related to shallow heating). The associated cooling curve is displayed in the right panel of Fig. S5. Our cooling model with gapless superfluidity reproduces the observations as well as the model assuming BCS superfluidity (with realistic neutron pairing [18]). However, the cooling model with gapless superfluidity leads to very different predictions that could be tested by future observations: the crust has not yet reached thermal equilibrium with the core and will further cool down during the next century (if no accretion occurs and if neutron vortices remain pinned, during this interval of time). Table S5 summarizes the median values of the parameters with 68% uncertainty level for both outburst I and outburst II.

### C. Neutron-star cooling models within the traditional model of accreted neutron stars

For comparison, we have performed cooling simulations within the traditional model of accreted neutron stars of Haensel & Zdunik [9], in which the diffusion of superfluid neutron stars in the crust is ignored.

#### *1. KS 1731−260*

Figure S9 shows the marginalized posterior probability distributions of the model parameters for KS 1731−260 in absence of superflow ($\mathbb{V}_n = 0$) and using the realistic neutron pairing gap of Ref. [18] (left panel) or the fine-tuned "Deep" gap of Ref. [15] (right panel). The median values of the model parameters with uncertainties at 68% level, summarized in Table S6, are consistent with those obtained in Ref. [13]. The associated cooling curves are shown in Fig. S10. Ignoring the presence of superflow as in previous studies, the cooling model with the realistic neutron pairing gap of Ref. [18] (dotted curve) fails to explain the late time cooling after $10^3$ days and leads to a rather poor fit of the earlier observations. The last four data points can only be reproduced by artificially fine tuning the neutron pairing gap [15] (dashed curve). In contrast, allowing for gapless superfluidity (solid curve) yields an excellent fit to the full data set. The marginalized posterior probability distributions for the cooling model assuming gapless superfluidity is shown in Fig. S11 and the median values of the parameters with uncertainties at 68% level are given in Table S6.

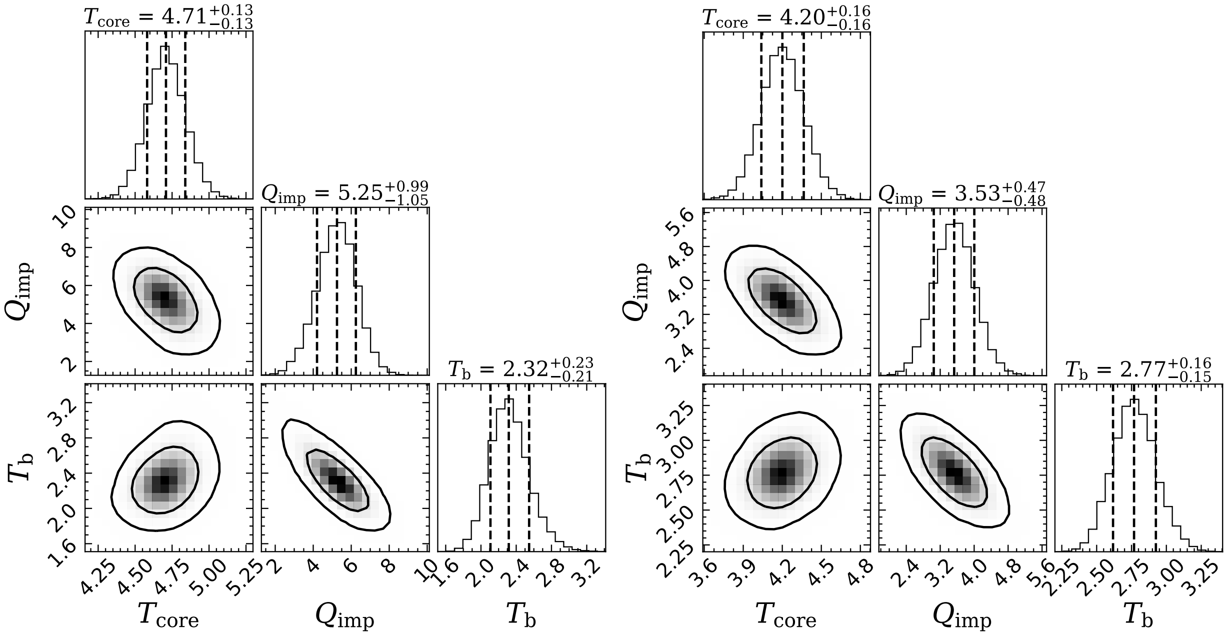


(a) QMC22 (b) Deep

FIG. S9: Marginalized 1-D and 2-D probability distributions for the parameters of our cooling model of KS 1731−260 within the traditional model of Haensel & Zdunik [9] of accreted neutron stars in the absence of superflow (BCS state). Results were obtained using the realistic neutron pairing gap of Ref. [18] (left panel) and the fine-tuned "Deep" gap of Ref. [15] (right panel). $T_{\rm core}$ and $T_{\rm b}$ are expressed in units of $10^7$ K and $10^8$ K respectively. The dotted lines in the histograms mark the median value and the 68% uncertainty level while the contours in the 2-D probability distributions correspond to 68% and 95% credibility ranges. The cooling curves corresponding to the median values of the parameters, are displayed in Fig. S10.

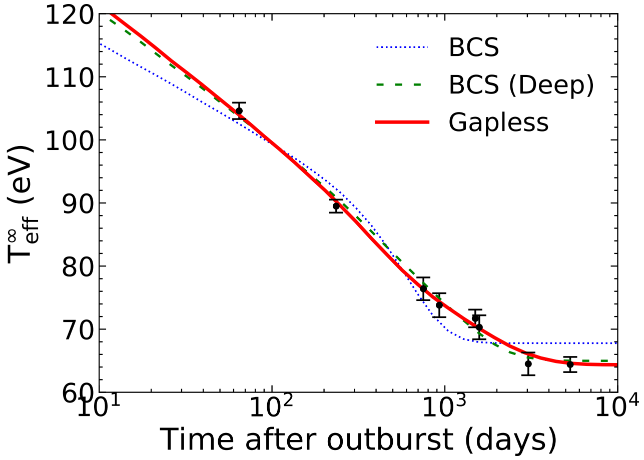


FIG. S10: Evolution of the effective surface temperature of KS 1731−260 in electronvolts (as seen by an observer at infinity) as a function of the time in days within the model of Haensel&Zdunik [9] of accreted neutron stars. Symbols represent observational data with error bars. The dotted and solid lines are models considering superfluid neutrons in the BCS and gapless states respectively using the realistic neutron pairing calculations of Ref. [18]. For comparison, results obtained with a model considering BCS superfluidity with the fine-tuned "Deep" gap of Ref. [15] are also shown (dashed line).

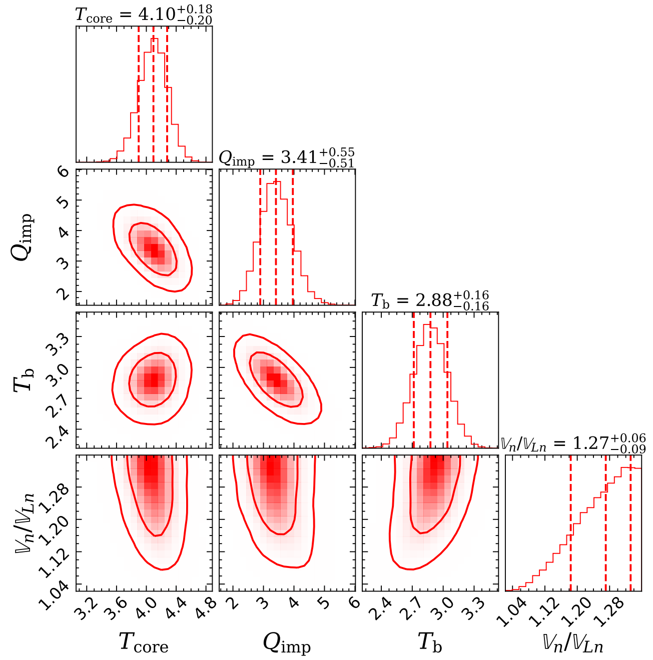


FIG. S11: Marginalized 1-D and 2-D probability distributions for the parameters of our cooling model of KS 1731−260 within the traditional model of Haensel&Zdunik [9] of accreted neutron stars but considering gapless superfluidity, using the realistic neutron pairing calculations of Ref. [18]. $T_{\rm core}$ and $T_{\rm b}$ are expressed in units of $10^7$ K and $10^8$ K respectively. The dotted lines in the histograms mark the median value and the 68% uncertainty level while the contours in the 2-D probability distributions correspond to 68% and 95% credibility ranges. The cooling curve corresponding to the median values of the parameters, is displayed in Fig. S10.

*2. MXB 1659−29*

Figure S12 shows the marginalized posterior probability distributions of the model parameters for the outburst I of MXB 1659−29 considering BCS superfluidity and using the realistic neutron pairing gap of Ref. [18] (left panel) or the fine-tuned "Deep" gap of Ref. [15] (right panel). The median values of the parameters with uncertainties at 68% are indicated in Table S7. The associated cooling curves are shown in the left panel of Fig. S13. With realistic pairing gaps, the neutron star was cooling so rapidly that thermal equilibrium was restored about $10^3$ days after the end of the outburst thus failing to reproduce the point at $k_{\rm B}T_{\rm eff}^{\infty} = 49 \pm 2$ eV. As previously shown in Ref. [15], a better fit can be obtained by artificially fine-tuning the pairing gap. This can be seen in Fig. S13 by comparing the cooling curves obtained with the realistic gap and the "Deep" gap.

As shown in Fig. S13 (left panel), the last observation can be reproduced with realistic pairing by considering gapless superfluidity. The marginalized posterior probability distributions are shown in the left panel of Fig. S15. The median values of the parameters with uncertainties at 68% are indicated in Table S7.

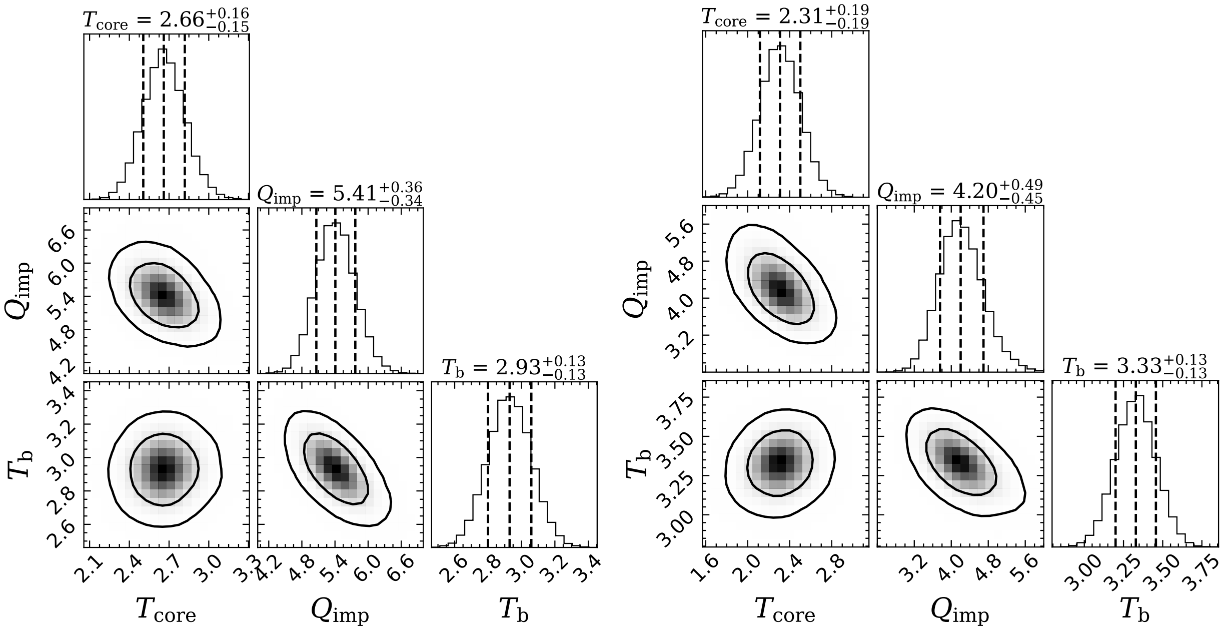


(a) QMC22 (b) Deep

FIG. S12: Marginalized 1-D and 2-D probability distributions for the parameters of our cooling model of the outburst I of MXB 1659-29 within the traditional model of Haensel&Zdunik [9] of accreted neutron stars in the absence of superflow (BCS state). Results were obtained using the realistic neutron pairing gap of Ref. [18] (left panel) and the fine-tuned "Deep" gap of Ref. [15] (right panel). $T_{\rm core}$ and $T_{\rm b}$ are expressed in units of $10^7$ K and $10^8$ K respectively. The dotted lines in the histograms mark the median value and the 68% uncertainty level while the contours in the 2-D probability distributions correspond to 68% and 95% credibility ranges. The cooling curves corresponding to the median values of the parameters, are displayed in the left panel of Fig. S13.

The marginalized posterior probability distributions of the model parameters for the outburst II assuming BCS superfluidity are shown in Fig. S14. Results obtained with gapless superfluidity are shown in Fig. S15 (right panel). Comparing the resulting cooling curves (right panel of Fig. S13), gapless superfluidity is found to better reproduce the observations. We find no significant change of $Q_{\rm imp}$ (consistent with the analysis of Ref. [2] assuming BCS superfluidity) and $\mathbb{V}_n$ at the 95% level, contrary to $T_{\rm b}$ (related to shallow heating).

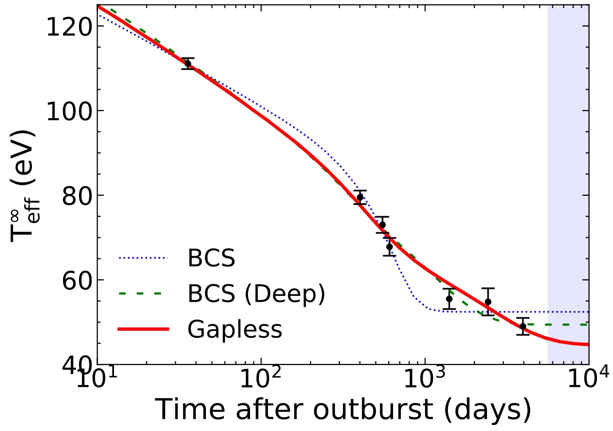


(a) Outburst I

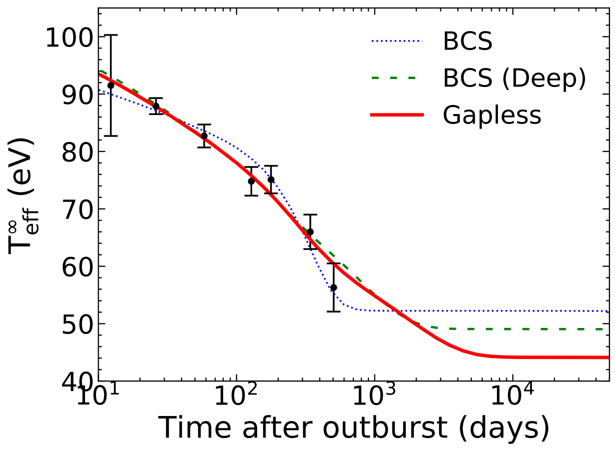


(b) Outburst II

FIG. S13: Evolution of the effective surface temperature of MXB 1659−29 (as seen by an observer at infinity) as a function of the time in days after outburst I (left panel) and outburst II (right panel) within the traditional model of Haensel&Zdunik [9] of accreted neutron stars but allowing for gapless superfluidity. Symbols represent observational data with error bars. $T_{\rm core}$ and $T_{\rm b}$ are expressed in units of $10^7$ K and $10^8$ K respectively. The dotted and solid lines are models considering superfluid neutrons in the BCS and gapless states respectively using the realistic neutron pairing calculations of Ref. [18]. For comparison, results obtained with a model considering BCS superfluidity with the fine-tuned "Deep" gap of Ref. [15] are also shown (dashed line). The shaded area corresponds to the second accretion phase (which occurred in 2015) and its subsequent cooling phase: the cooling curves within this region depict the expected behavior had the outburst II not occurred.

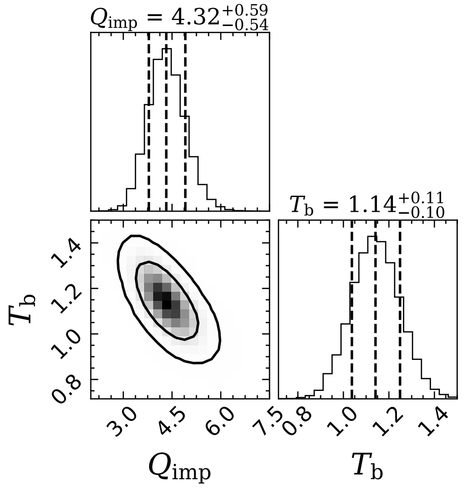


(a) QMC22

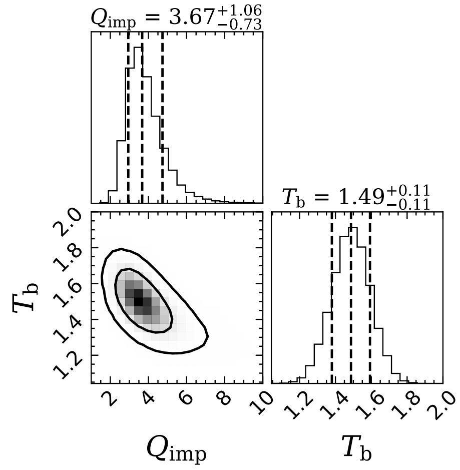


(b) Deep

FIG. S14: Same as Fig. S12 for the outburst outburst II of MXB 1659-29. The cooling curves corresponding to the median values of the parameters, are displayed in the right panel of Fig. S13.

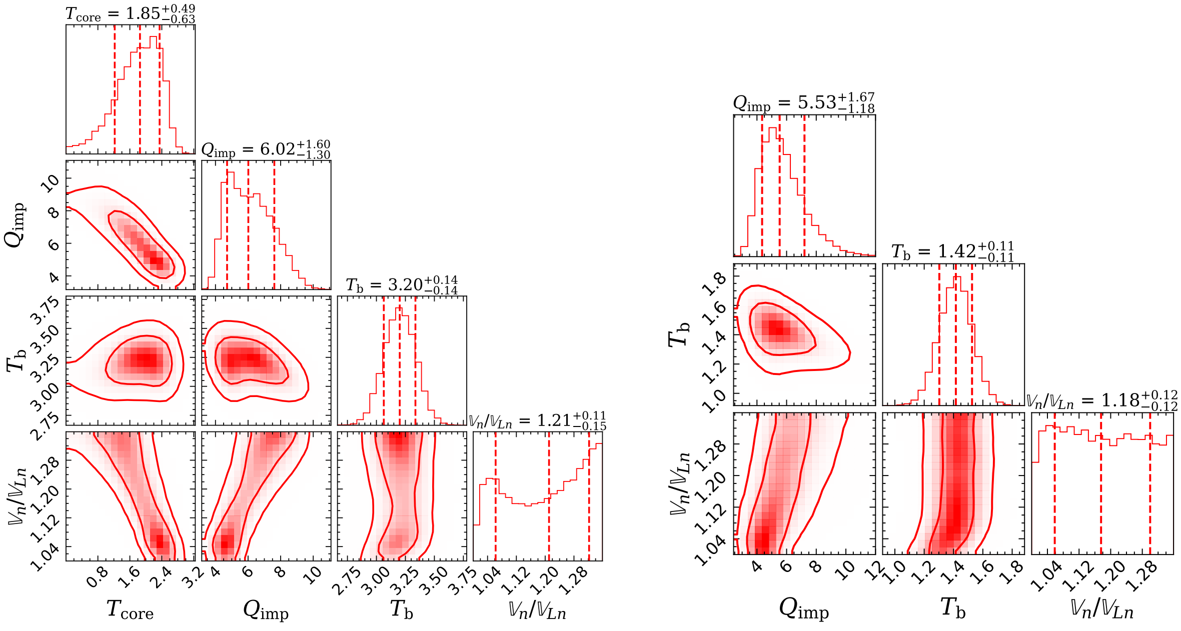


(a) Outburst I (b) Outburst II

FIG. S15: Marginalized 1-D and 2-D probability distributions for the parameters of our cooling model of the outburst I (left panel) and outburst II (right panel) of MXB 1659−29 within the traditional model of Haensel&Zdunik [9] of accreted neutron stars in the presence of gapless superfluidity, using the realistic neutron pairing calculations of Ref. [18]. $T_{\rm core}$ and $T_{\rm b}$ are expressed in units of $10^7$ K and $10^8$ K respectively. The dotted lines in the histograms mark the median value and the 68% uncertainty level while the contours in the 2-D probability distributions correspond to 68% and 95% credibility ranges. The cooling curves corresponding to the median values of the parameters, are displayed in Fig. S13.

### D. Neutron superfluidity and cooling

To better understand the role of free neutrons, we have plotted in Fig. S16 the different contributions to the specific heat of the crust for MXB 1659−29 (for outburst I, left panel) and for KS 1731−260 (right panel) within the model of accreted neutron stars of Refs. [10, 11]. The parameters are given by the median values in panel (a) of Fig. S8 and Fig. S7, namely : $\mathbb{V}_n/\mathbb{V}_{Ln} = 1.23$, $Q_{\rm imp} = 17.16$, $T_{\rm core} = 0.85 \times 10^7$ K, and $T_{\rm b} = 3.14 \times 10^8$ K for MXB 1659−29 and $\mathbb{V}_n/\mathbb{V}_{Ln} = 1.21$, $Q_{\rm imp} = 5.80$, $T_{\rm core} = 3.99 \times 10^7$ K, and $T_{\rm b} = 3.13 \times 10^8$ K for KS 1731−260. Calculations were made using the realistic neutron pairing calculations of Ref. [18]. Results for outburst II of MXB 1659−29 are very similar to those obtained for outburst I and are not displayed. In the absence of superflow, the neutron contribution calculated with realistic pairing gap is completely negligible compared to that of electrons and is thus not displayed in Fig. S16. For this reason, the neutron-star cooling curves are essentially independent of the adopted values for $\Delta_n^{(0)}$ (however, this is not the case for the fine-tuned gaps). In the gapless state, the neutron specific heat is comparable to that in the normal phase and dominates by one or two orders of magnitude the contributions due to electrons and ions in all crustal layers. Because the neutron specific heat is then a universal function of $\mathbb{V}_n/\mathbb{V}_{Ln}$, the cooling curves obtained for given ratios $\mathbb{V}_n/\mathbb{V}_{Ln}$ are the same for the different realistic calculations of $\Delta_n^{(0)}$. It is only in the limiting case $\mathbb{V}_n = \mathbb{V}_{Ln}$ that the cooling curves exhibit some small variations with respect to $\Delta_n^{(0)}$. The enhancement of the crustal specific heat leads to a delayed thermal relaxation. This can be easily understood recalling that the thermal relaxation time of the crust is roughly given by [26]

$$\tau \sim \frac{c_V^{\rm crust}}{\kappa_{\rm crust}} \Delta R^2 \tag{S.4}$$

where $c_V^{\rm crust}$ and $\kappa_{\rm crust}$ denote the specific heat and the thermal conductivity of the crust respectively, and $\Delta R$ is the crust thickness.

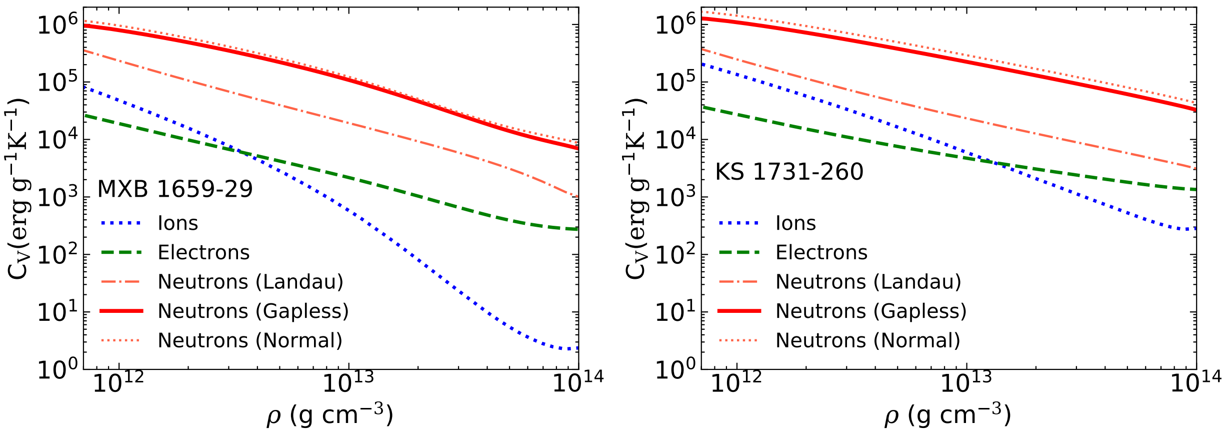


FIG. S16: Specific heat contributions in erg g$^{-1}$ K$^{-1}$ as a function of the average mass density (in g cm$^{-3}$) in the inner crust of the neutron stars MXB 1659−29 at the end of outburst I (left panel) and KS 1731−260 (right panel). In the BCS state ($\mathbb{V}_n = 0$), the neutron contribution is not shown since it is negligible compared to the ion (blue dotted curve) and electron (green dashed curve) contributions. In the gapless state, the neutron contribution (red solid curve) gives the main contribution to the crustal specific heat. For comparison, we have also plotted the neutron specific heat for Landau's effective superfluid velocity $\mathbb{V}_n = \mathbb{V}_{Ln}$ (red dotted-dashed curve). The neutron specific heat in the normal phase at the critical effective superfluid velocity $\mathbb{V}_n = {\rm e}\mathbb{V}_{Ln}/2$ is represented by the red dotted curve.

The reduction factor $R_{00}^{\rm (Gapless)}$ we used for the gapless state in our simulations was derived under the assumption of low temperatures $T \ll T_{cn}^{(0)}$. The highest temperatures $\sim 0.05 T_{cn}^{(0)}$ are reached in KS 1731−260 at the end of the outburst in the shallowest layers of the inner crust at densities $10^{11} - 10^{12}$ g cm$^{-3}$, as illustrated in Fig. S17. Computing the neutron specific heat numerically from the general expression given in Ref. [22], we find that the errors are at most 0.56% for KS 1731−260 and 0.18% for MXB 1659−29 (after the end of outburst I). For the deeper layers of relevance for the late time cooling, $T \sim 10^{-2} T_{cn}^{(0)}$ therefore the errors on the neutron specific heat are considerably reduced (they do not exceed 0.021% for both KS 1731−260 and MXB 1659−29). A systematic study of the errors

can be found in Ref. [22]. Let us stress that those estimated errors are upper limits and rapidly decrease as the crust cools down.

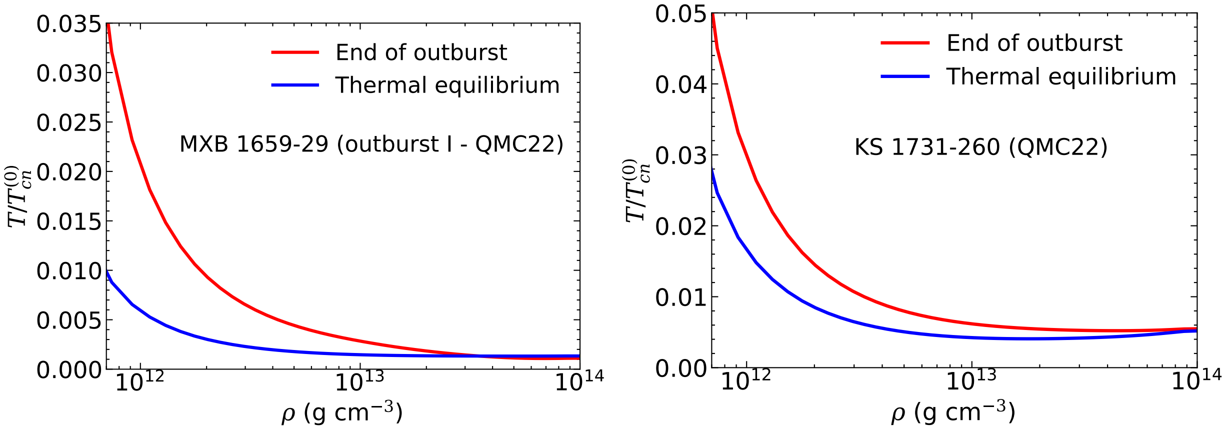


FIG. S17: Temperature (in units of $T_{cn}^{(0)}$) in the inner crust of MXB 1659−29 (outburst I, left panel) and KS 1731−260 (right panel) at the end of the accretion phase (red curves) and after the thermal equilibrium between the crust and the core was restored (blue curves) using our best model considering gapless superfluidity.

## S.V. SUMMARY OF THE RESULTS

### A. Thermodynamically consistent model

Here we report the results obtained within the thermodynamically consistent model of accreted neutron stars of Gusakov&Chugunov [10, 11]. Quantities that have been kept fixed during MCMC simulations are denoted in bold.

TABLE S4: Results for KS 1731−260 within the model of Gusakov&Chugunov [10, 11] of accreted neutron stars considering BCS ($\mathbb{V}_n = 0$) or gapless ($\mathbb{V}_{cn}^{(0)} \geq \mathbb{V}_n \geq \mathbb{V}_{Ln}$) superfluidity. Median values of the model parameters are displayed with 68% uncertainty level. The labels "QMC22" and "Deep" refer to the realistic neutron pairing gap of Refs. [18] and the fine-tuned neutron pairing gap of Ref. [15], respectively.

| Neutron pairing | $T_{\rm core}$ ($10^7$K) | $Q_{\rm imp}$ | $T_{\rm b}$ ($10^8$K) | $\mathbb{V}_n/\mathbb{V}_{Ln}$ |
|---|---|---|---|---|
| QMC22 | 4.69±0.14 | $10.56^{+2.15}_{-1.97}$ | $2.45^{+0.19}_{-0.18}$ | **0** |
| Deep | 4.13±0.18 | $4.78^{+0.84}_{-0.77}$ | $3.22^{+0.14}_{-0.15}$ | **0** |
| QMC22 | $3.99^{+0.26}_{-0.34}$ | $5.80^{+1.68}_{-1.25}$ | $3.13^{+0.19}_{-0.20}$ | $1.21^{+0.10}_{-0.11}$ |

TABLE S5: Results for MXB 1659−29 within the model of Gusakov&Chugunov [10, 11] of accreted neutron stars, considering BCS ($\mathbb{V}_n = 0$) or gapless ($\mathbb{V}_{cn}^{(0)} \geq \mathbb{V}_n \geq \mathbb{V}_{Ln}$) superfluidity. Median values of the model parameters are displayed with 68% uncertainty level, and have been obtained using the realistic neutron pairing gap of Ref. [18] (labelled as "QMC22") or the fine-tuned "Deep" gap of Ref. [15].

| Outburst | Neutron pairing | $T_{\rm core}$ ($10^7$K) | $Q_{\rm imp}$ | $T_{\rm b}$ ($10^8$K) | $\mathbb{V}_n/\mathbb{V}_{Ln}$ |
|---|---|---|---|---|---|
| I | QMC22 | 2.69±0.15 | $8.05^{+0.71}_{-0.61}$ | 3.11±0.13 | **0** |
| II | QMC22 | **2.69** | $8.17^{+1.55}_{-1.28}$ | $1.40^{+0.10}_{-0.09}$ | **0** |
| I | Deep | $0.67^{+0.64}_{-0.46}$ | $15.27^{+2.45}_{-2.72}$ | $3.19^{+0.16}_{-0.15}$ | **0** |
| II | Deep | **0.67** | $30.77^{+11.42}_{-8.00}$ | $1.36^{+0.12}_{-0.11}$ | **0** |
| I | QMC22 | $0.85^{+0.59}_{-0.54}$ | $17.16^{+3.49}_{-3.70}$ | $3.14^{+0.16}_{-0.15}$ | $1.23^{+0.09}_{-0.11}$ |
| II | QMC22 | **0.85** | $26.53^{+10.86}_{-8.09}$ | 1.38±0.11 | 1.18±0.12 |

### B. Traditional model

Here we report the results obtained within the traditional model of accreted neutron stars of Haensel&Zdunik [9], in which the diffusion of superfluid neutrons in the crust is ignored. Quantities that have been kept fixed during MCMC simulations are denoted in bold.

TABLE S6: Results for KS 1731−260 within the traditional model of Haensel&Zdunik [9] of accreted neutron stars, considering BCS ($\mathbb{V}_n = 0$) or gapless ($\mathbb{V}_{cn}^{(0)} \geq \mathbb{V}_n \geq \mathbb{V}_{Ln}$) superfluidity. Median values of the model parameters are displayed with 68% uncertainty level. The labels "QMC22" and "Deep" refer to the realistic neutron pairing gap of Refs. [18] and the fine-tuned neutron pairing gap of Ref. [15], respectively.

| Neutron pairing | $T_{\rm core}$ ($10^7$K) | $Q_{\rm imp}$ | $T_{\rm b}$ ($10^8$K) | $\mathbb{V}_n/\mathbb{V}_{Ln}$ |
|---|---|---|---|---|
| QMC22 | 4.71±0.13 | $5.25^{+0.99}_{-1.05}$ | $2.32^{+0.23}_{-0.21}$ | **0** |
| Deep | 4.20±0.16 | $3.53^{+0.47}_{-0.48}$ | $2.77^{+0.16}_{-0.15}$ | **0** |
| QMC22 | $4.10^{+0.18}_{-0.20}$ | $3.41^{+0.55}_{-0.51}$ | 2.88±0.16 | $1.27^{+0.06}_{-0.09}$ |

TABLE S7: Results for MXB 1659−29 within the traditional model of Haensel&Zdunik [9] of accreted neutron stars, considering BCS ($\mathbb{V}_n = 0$) or gapless ($\mathbb{V}_{cn}^{(0)} \geq \mathbb{V}_n \geq \mathbb{V}_{Ln}$) superfluidity. Median values of the model parameters are displayed with 68% uncertainty level, and have been obtained using the realistic neutron pairing gap of Ref. [18] (labelled as "QMC22") or the fine-tuned "Deep" gap of Ref. [15].

| Outburst | Neutron pairing | $T_{\rm core}$ ($10^7$K) | $Q_{\rm imp}$ | $T_{\rm b}$ ($10^8$K) | $\mathbb{V}_n/\mathbb{V}_{Ln}$ |
|---|---|---|---|---|---|
| I | QMC22 | $2.66^{+0.16}_{-0.15}$ | $5.41^{+0.36}_{-0.34}$ | 2.93±0.13 | **0** |
| II | QMC22 | **2.66** | $4.32^{+0.59}_{-0.54}$ | $1.14^{+0.11}_{-0.10}$ | **0** |
| I | Deep | 2.31±0.19 | $4.20^{+0.49}_{-0.45}$ | 3.33±0.13 | **0** |
| II | Deep | **2.31** | $3.67^{+1.06}_{-0.73}$ | 1.49±0.11 | **0** |
| I | QMC22 | $1.85^{+0.49}_{-0.63}$ | $6.02^{+1.60}_{-1.30}$ | 3.20±0.14 | $1.21^{+0.11}_{-0.15}$ |
| II | QMC22 | **1.85** | $5.53^{+1.67}_{-1.18}$ | 1.42±0.11 | 1.18±0.12 |


[1] R. L. Merritt, E. M. Cackett, E. F. Brown, D. Page, A. Cumming, N. Degenaar, A. Deibel, J. Homan, J. M. Miller, and R. Wijnands, Astrophys. J. **833**, 186 (2016).
[2] Parikh, A. S., Wijnands, R., Ootes, L. S., Page, D., Degenaar, N., Bahramian, A., Brown, E. F., Cackett, E. M., Cumming, A., Heinke, C., et al., Astron. Astrophys. **624**, A84 (2019).
[3] E. Cackett, E. Brown, A. Cumming, N. Degenaar, J. K. Fridriksson, J. Homan, J. Miller, and R. Wijnands, Astrophys. J. **774**, 131 (2013).
[4] C. J. Horowitz, D. K. Berry, C. M. Briggs, M. E. Caplan, A. Cumming, and A. S. Schneider, Phys. Rev. Lett. **114**, 031102 (2015).
[5] A. Deibel, A. Cumming, E. F. Brown, and S. Reddy, Astrophys. J. **839**, 95 (2017).
[6] A. Y. Potekhin and G. Chabrier, Astron. Astrophys. **645**, A102 (2021).
[7] X. Y. Lu, G. L. Lü, H. L. Liu, C. H. Zhu, and Z. J. Wang, Res. Astron. Astrophys. **22**, 055018 (2022).
[8] A. Y. Potekhin, M. E. Gusakov, and A. I. Chugunov, Mon. Not. R. Astron. Soc. **522**, 4830 (2023), ISSN 0035-8711.
[9] P. Haensel and J. L. Zdunik, Astron. Astrophys. **227**, 431 (1990).
[10] M. E. Gusakov and A. I. Chugunov, Phys. Rev. Lett. **124**, 191101 (2020).
[11] M. E. Gusakov and A. I. Chugunov, Phys. Rev. D **103**, L101301 (2021).
[12] F. Douchin and P. Haensel, Astron. Astrophys. **380**, 151 (2001).
[13] E. F. Brown and A. Cumming, Astrophys. J. **698**, 1020 (2009).
[14] K. P. Levenfish and D. G. Yakovlev, Astron. Rep. **38**, 247 (1994).
[15] Turlione, A., Aguilera, D. N., and Pons, J. A., Astron. Astrophys. **577**, A5 (2015).
[16] A. Schwenk, B. Friman, and G. E. Brown, Nucl. Phys. A **713**, 191 (2003).
[17] S. Gandolfi, A. Y. Illarionov, S. Fantoni, F. Pederiva, and K. E. Schmidt, Phys. Rev. Lett. **101**, 132501 (2008).
[18] S. Gandolfi, G. Palkanoglou, J. Carlson, A. Gezerlis, and K. E. Schmidt, Condensed Matter **7** (2022).
[19] L. G. Cao, U. Lombardo, C. W. Shen, and N. V. Giai, Phys. Rev. C **73**, 014313 (2006).

[20] M. Drissi and A. Rios, Eur. Phys. J. A **58**, 90 (2022).
[21] E. Krotscheck, P. Papakonstantinou, and J. Wang, Astrophys. J. **955**, 76 (2023).
[22] V. Allard and N. Chamel, Phys. Rev. C **108**, 015801 (2023).
[23] D. Foreman-Mackey, D. W. Hogg, D. Lang, and J. Goodman, PASP **125**, 306 (2013), 1202.3665.
[24] P. C. Gregory, Astrophys. J. **631**, 1198 (2005).
[25] A. Gelman and D. B. Rubin, Statistical Science **7**, 457 (1992).
[26] D. Page and S. Reddy, Phys. Rev. Lett. **111**, 241102 (2013).
